# Supplementary material for: User-Friendly Safety Monitoring System for Manufacturing Cobots
Source: arXiv:2307.01886 source file (2023-07-04)
Supplement: Supplementary file 1 [file Appendix.tex]

\section{Appendix}
\label{sec:append}
Not provided in the submitted version
